# Supplementary material for: 3D Concept Learning and Reasoning from Multi-View Images
Source: arXiv:2303.11327 source file (2023-03-20)
Supplement: Supplementary file 1 [file _supplementary.tex]

\input{_constants}
\review % \review OR \cameraready

\documentclass[10pt,twocolumn,letterpaper]{article}
\input{cvpr_header}
\myexternaldocument{_main}
\begin{document}
%% TITLE
\title{\paperTitle \\ Supplemental Material}
\author{\authorBlock}
\maketitle
%%

%%
%{
%    \hypersetup{linkcolor=black}
%    \tableofcontents
%}
%\clearpage

\input{12_appendix}

{\small
\bibliographystyle{ieee_fullname}
\bibliography{11_references}
}

\end{document}
